# Supplementary material for: Cross-lingual Parsing with Polyglot Training and Multi-treebank Learning: A Faroese Case Study
Source: arXiv:1910.07938 source file (2019-10-17)
Supplement: Supplementary file 1 [file appendix.tex]

\appendix
\section{Supplemental Material}
\label{sec:supplemental}
Supplementary material should be uploaded as separate files when submitting the paper for review. Upon acceptance, the appendices come after the references without a page break.

\section{Parser Details}
\input{parser-details.tex}
